# Supplementary material for: Causal Graph Learning via Distributional Invariance of Cause-Effect Relationship
Source: arXiv:2602.03353 source file (2026-02-03)
Supplement: Supplementary file 1 [file supp-iclr-discussion.tex]

\hung{\subsection{On the intuition of minimal downsampling rate}
The intuition of the minimal downsampled rate is mentioned in the first two paragraphs of Section 4.2.2. To further elaborate, our invariance test requires drawing samples Di from the augmented distribution $P_i(\boldsymbol{B})$ of the true oracle $P(\boldsymbol{X})$. This cannot be done directly as explained above, we achieve this via drawing a sample $D_i$ from $D$, which is supposed to preserve $D$'s evidence of all (hidden) cause-effect relationships.}

\hung{As such, $D_i$ cannot contain duplicated data points from $D$ because otherwise, it might (statistically) emphasize on (incorrect) cause-effect relationships that were not implied by $D$ and hence, $P_i$. Thus, $D_i$ must be a downsample. But, a downsample might lose information so we want to minimize $|D|/|D_i|$ which stipulates the maximum size of $|D_i|$ at which we can still guarantee $D_i \sim P_i(\boldsymbol{X})$. This rate is computable via Theorem 4 -- see Eq. (4).
}

\hung{
\subsection{On the application to time-series and heterogeneous data}
In principle, our proposed causal discovery algorithm should work for (multivariate) time-series data which is also underlied by an (unknown) Bayesian Network reflecting its causal relationship. In practice, we foresee a (practical) challenge in terms of scalability. To elaborate, the size of the causal graph scales linearly in the number of time steps. Hence, for $d$-variable cases, the total number of nodes in the corresponding Bayesian Net of the whole $T$ timesteps is $O(dT)$. As the complexity of our proposal is $O(|node|^2)$, its complexity will grow quadratically in the number of time steps which will cause scalability issues since $T$ can be very large. Thus, the key challenge in extending this to time-series data is scalability.}

\hung{Our proposed method can also handle multiple heterogeneous datasets sharing the same causal graph (albeit with different sets of effect-cause conditional distributions). In this case, the invariant test can be slightly repurposed to simply find the plausible parent set with minimal variance (see Equation~\ref{eq:invariance}) across those datasets. We have in fact conducted a preliminary study in this setting in Appendix~\ref{supp:distributed}.
}
