# Supplementary material for: Causal Graph Learning via Distributional Invariance of Cause-Effect Relationship
Source: arXiv:2602.03353 source file (2026-02-03)
Supplement: Supplementary file 2 [file supp-iclr-sachs.tex]

\subsection{Evaluation on the golden standard -- SACHS dataset (2005)}
As per constructive suggestions from the reviewers, in this section, we evaluate our proposal \textbf{GLIDE} in comparison to the state-of-the-art baselines on the SACHS dataset provided by \cite{sachs-data}. This dataset has been widely used in many existing literatures on causal discovery \cite{zheng2018dags, zheng2020learning}. This dataset consists of continuous measurements of expression levels of proteins and phospholipids in human immune system cells and is widely accepted by the biology community. The SACHS graph contains $11$ variables and $17$ edges. The results are reported (mean and $95\%$-confidence interval after $10$ independent runs) as in Table~\ref{tab:sachs} where TPR (true positive rate -- the ratio of true causal edges in the output graph) is included.

The reported results show that \textbf{GLIDE} significantly outperforms other baselines, achieving the lowest SHD ($8.7\pm0.48$) and spurious rate ($0\%$). When compared to the second-best baseline (SCORE), \textbf{GLIDE} notably almost doubles the TPR of SCORE ($83\%$ verses $49\%$) while running three times faster. In contrast, GIES finishes the causal finding procedure within $3$ seconds, but the output graph contains $57\%$ of spurious relationships, which amounts to over $3$ times higher SHD than \textbf{GLIDE}.

\begin{table}[tb]
\centering
\caption{Comparison on the real-world standardized SACHS dataset.}
\label{tab:sachs}
\begin{tabular}{|lllll|}
\hline
\multicolumn{1}{|c}{\textbf{Baselines}} &
  \multicolumn{1}{c}{\textbf{SHD}} &
  \multicolumn{1}{c}{\textbf{\begin{tabular}[c]{@{}c@{}}Spurious\\ rate\end{tabular}}} &
  \multicolumn{1}{c}{\textbf{TPR}} &
  \multicolumn{1}{c|}{\textbf{\begin{tabular}[c]{@{}c@{}}RunTime\\ (seconds)\end{tabular}}} \\ \hline\hline
\textbf{GLIDE}      & $\color{red}8.7 \pm 0.48$   & $\color{red}0.00 \pm 0.00$       & $\color{red}0.83 \pm 0.05$ & $10.46 \pm 0.71$   \\ \hline
DAS        & $22.27 \pm 1.65$ & $0.55 \pm 0.04$ & $0.24 \pm 0.03$ & $16.45 \pm 4.23$   \\ \hline
SCORE      & $13.2 \pm 0.66$  & $0.22 \pm 0.04$ & $0.49 \pm 0.04$ & $30.02 \pm 3.98$   \\ \hline
FCI        & $17.00 \pm 0.00$       & $0.44 \pm 0.00$    & $0.33 \pm 0.00$    & $4.06 \pm 0.63$    \\ \hline
GIES       & $27.00 \pm 0.00$       & $0.57 \pm 0.00$    & $0.15 \pm 0.00$    & $\color{red}2.69 \pm 0.12$    \\ \hline
Notears    & $51.00 \pm 0.00$       & $0.69 \pm 0.00$    & $0.09 \pm 0.00$    & $575.97 \pm 14.11$ \\ \hline
MLPNotears & $43.33 \pm 4.77$ & $0.66 \pm 0.03$ & $0.15 \pm 0.01$ & $164.86 \pm 12.73$ \\ \hline
\end{tabular}
\end{table}
